# Supplementary material for: Trustworthy AI in practice: an analysis of practitioners' needs and challenges
Source: arXiv:2407.12135 source file (2024-05-15)
Supplement: Supplementary file 1 [file 8_Appendix.tex]

\section{Appendix}
\label{sec:appendix}

\begin{table*}[t]
\caption{Interviewees' self-reported technology areas and team roles. Interviewees whose ID starts with \textbf{T} are the ones with whom we tested the interview; \textbf{P} are the formal participants. The roles are: Researcher (Researcher); Software Engineer / Developer (SED), Technical Lead / Manager (TLM), Project Lead / Project Manager (PLM), Product Manager (PM), Executive / General Manager (EGM), Domain / Content Expert (DCE), Data Scientist (DS).}
\label{table:formal_interview_subjects}
\small
%\begin{tabular}{|c|l|l|}
\begin{tabular}{l l l}
\hline
\multicolumn{1}{l}{\textbf{Technology Area}}            & \textbf{Roles of Interviewees} & \textbf{Interviewee ID} \\ \hline
Recommender Systems, Automotive IDS & Researcher                                                                                                                                                             & T1                                                                                                             \\
Computer Vision / Image Analysis    & Researcher                                                                                                                                                             & T2                                                                                                             \\ \hline
Computer Vision / Image Analysis    & \begin{tabular}[c]{@{}l@{}}Researcher,SED,TLM,PLM/PM\end{tabular} & \begin{tabular}[c]{@{}l@{}}P1,P2,P4,P10,P11, P12,P13,P14,P15,\\P18,P23,P26,P32\end{tabular}                 \\ \hline
Conversational AI / Chatbots        & \begin{tabular}[c]{@{}l@{}}Researcher,PLM/PM,TLM,EGM\end{tabular}   & \begin{tabular}[c]{@{}l@{}}P1,P17,P18,P21,P29,P30,P31,P32\end{tabular}                                      \\ \hline
Natural Language Processing         & \begin{tabular}[c]{@{}l@{}}Researcher,TLM,DCE,TLM,EGM\end{tabular}   & \begin{tabular}[c]{@{}l@{}}P1,P2,P6,P9,P13,P14,P15,P16,P18,P20,P29,\\P30,P31,P32\end{tabular}              \\ \hline
Robotics / Cyber-physical Systems   & Researcher                                                                                                                                                             & P1,P10,P14                                                                                                     \\ \hline
Search / Information Retrieval      & \begin{tabular}[c]{@{}l@{}}Researcher,SED,TLM\end{tabular}                                                        & \begin{tabular}[c]{@{}l@{}}P3,P9,P12,P13,P26,P29,P30,P32,P33\end{tabular}                                   \\ \hline
Decision support                    & \begin{tabular}[c]{@{}l@{}}Researcher,TLM,DCE,PLM/PM\end{tabular}       & \begin{tabular}[c]{@{}l@{}}P4,P5,P13,P14,P15,P16,P17,P18,P19,\\P21,P24,P25,P27,P29,P30,P34\end{tabular} \\ \hline
Human Aspect                        & Researcher                                                                                                                                                             & P7                                                                                                             \\ \hline
Cyber-Security                      & Researcher                                                                                                                                                             & P8                                                                                                             \\ \hline
Recommender Systems                 & \begin{tabular}[c]{@{}l@{}}Researcher,TLM\end{tabular}                                                                                         & \begin{tabular}[c]{@{}l@{}}P13,P14,P15,P18,P19,P21,P22,P25,\\ P29,P33,P34\end{tabular}                      \\ \hline
Speech and Voice                    & \begin{tabular}[c]{@{}l@{}}Researcher,TLM\end{tabular}                                                                                        & P19,P29,P32,P33                                                                                                \\ \hline
User Modeling / Adaptive Hypermedia & Researcher                                                                                                                                                             & P20,P25,P33                                                                                                    \\ \hline
Other - Telemonitoring              & DS                                                                                                                                                         & P28                                                                                                            \\ \hline
\end{tabular}
\end{table*}

\begin{table}[t]
\caption{Participants grouped by company size.}
\label{tab:company_size}
\begin{tabular}{lc}
\hline
\textbf{Company size}     & \textbf{Count} \\ \hline
1-10 employees            & 7              \\ \hline
11-50 employees           & 4              \\ \hline
51-500   employees        & 8              \\ \hline
501-1000 employees        & 4              \\ \hline
More than 1,000 employees & 11             \\ \hline
\end{tabular}
\end{table}

\begin{table}[t]
\caption{Participants grouped by years of experience in their current role and in developing AI-enabled systems.}
\label{tab:years_experience}
\begin{tabular}{lcc}
\hline
\textbf{Years}        & \multicolumn{1}{c}{\textbf{\begin{tabular}[c]{@{}c@{}}Experience\\ in their \\ role\end{tabular}}} & \multicolumn{1}{c}{\textbf{\begin{tabular}[c]{@{}c@{}}Experience in \\ developing \\ AI-enabled\\ systems\end{tabular}}} \\ \hline
0-2 (junior)          & 13                                                                                                 & 11                                                                                                                       \\ \hline
3-5 (mid-experienced) & 13                                                                                                 & 14                                                                                                                       \\ \hline
6-10 (senior)         & 6                                                                                                  & 6                                                                                                                        \\ \hline
10+                   & 2                                                                                                  & 2                                                                                                                        \\ \hline
\end{tabular}
\end{table}
